# Supplementary material for: A General Theory for Federated Optimization with Asynchronous and Heterogeneous Clients Updates
Source: arXiv:2206.10189 source file (2022-06-21)
Supplement: Supplementary file 1 [file additional_exp.tex]

\section{Additional Experiments}\label{app:sec:experiments}

\begin{figure}
	\centering
	\includegraphics[width=\linewidth]{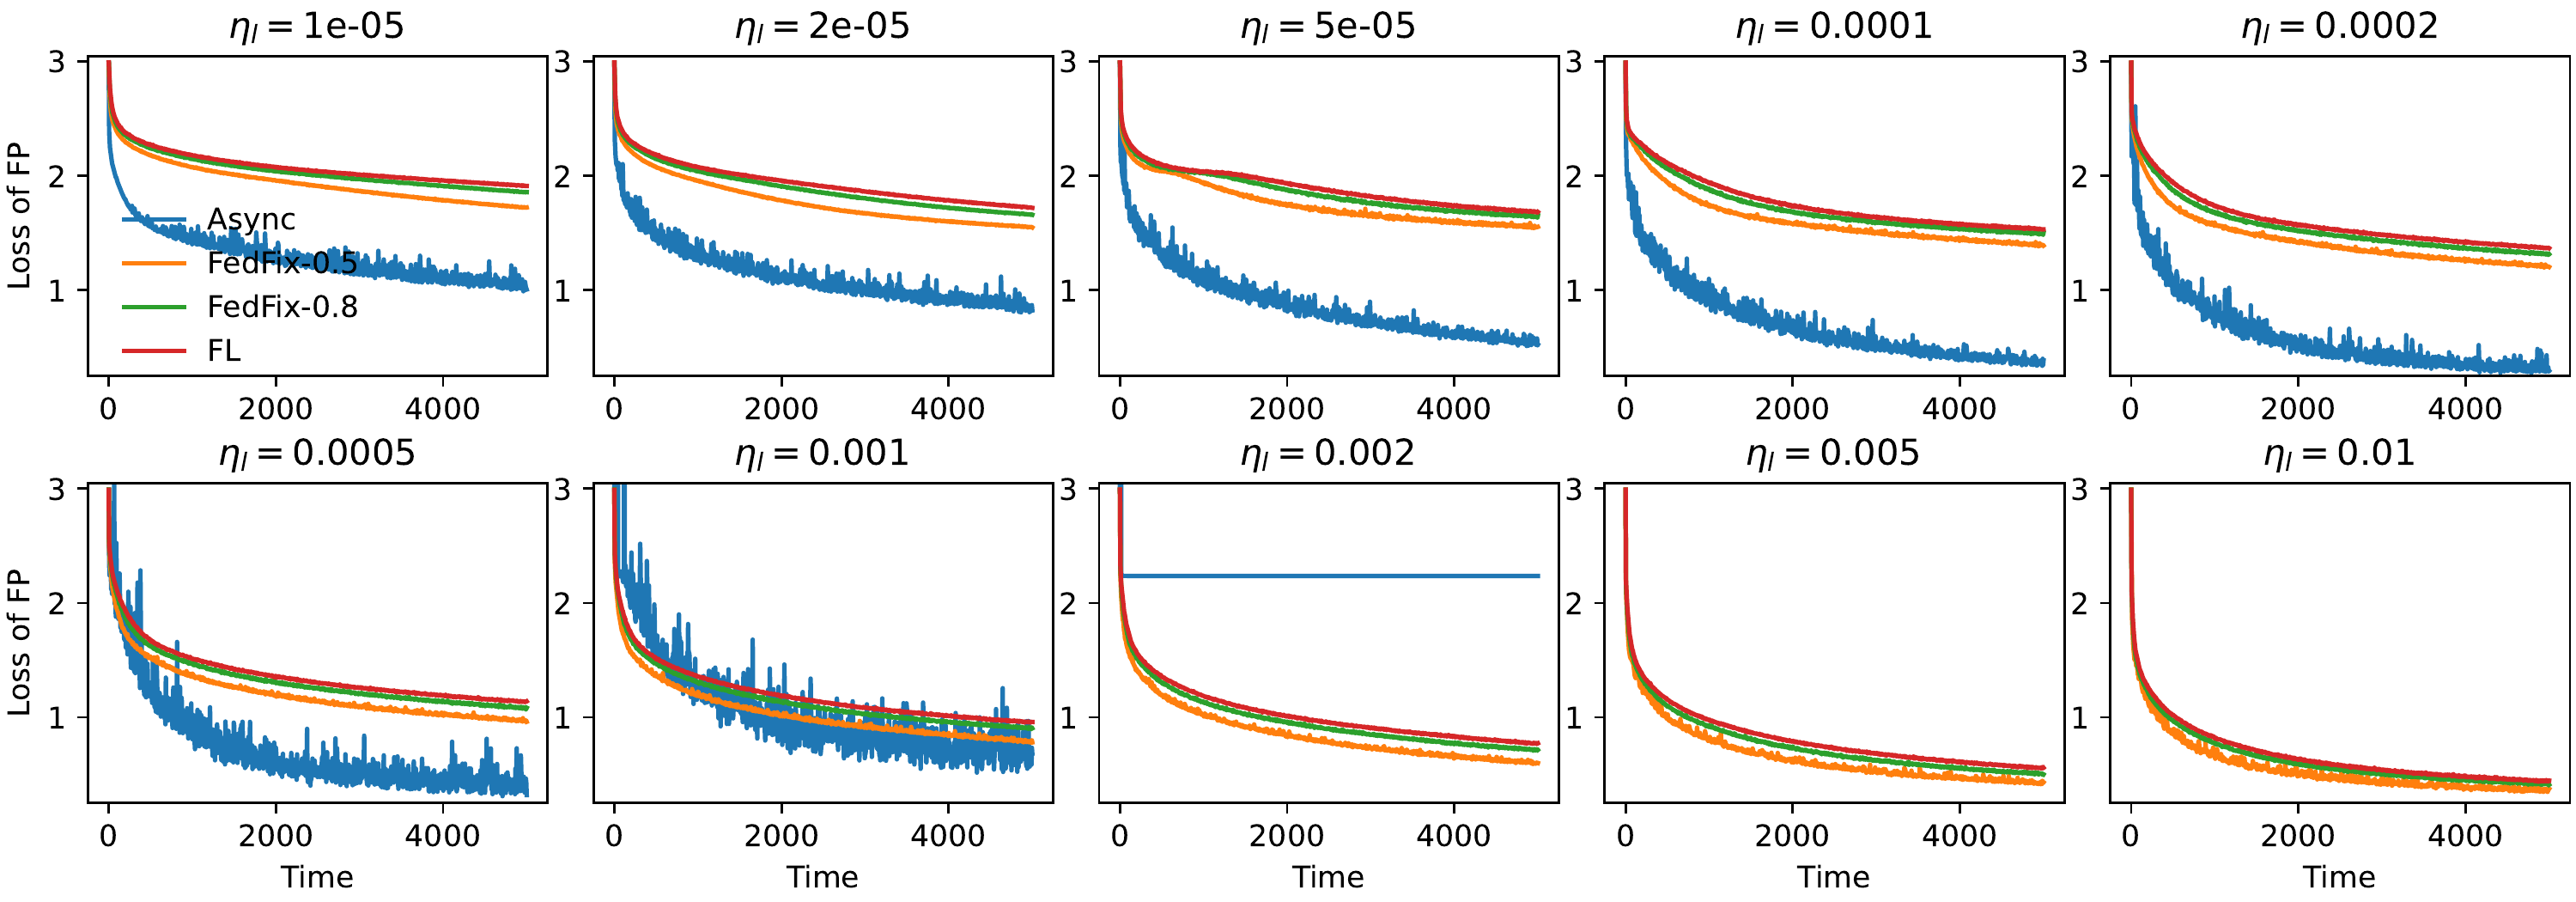}
	\caption{Evolution of federated problem (\ref{eq:original_problem_general}) loss for CIFAR10 and time scenario $F80$ with $M=20$ and $K=10$.}
	\label{app:fig:explore_CIFAR10_20}
\end{figure}

\begin{figure}
	\centering
	\includegraphics[width=\linewidth]{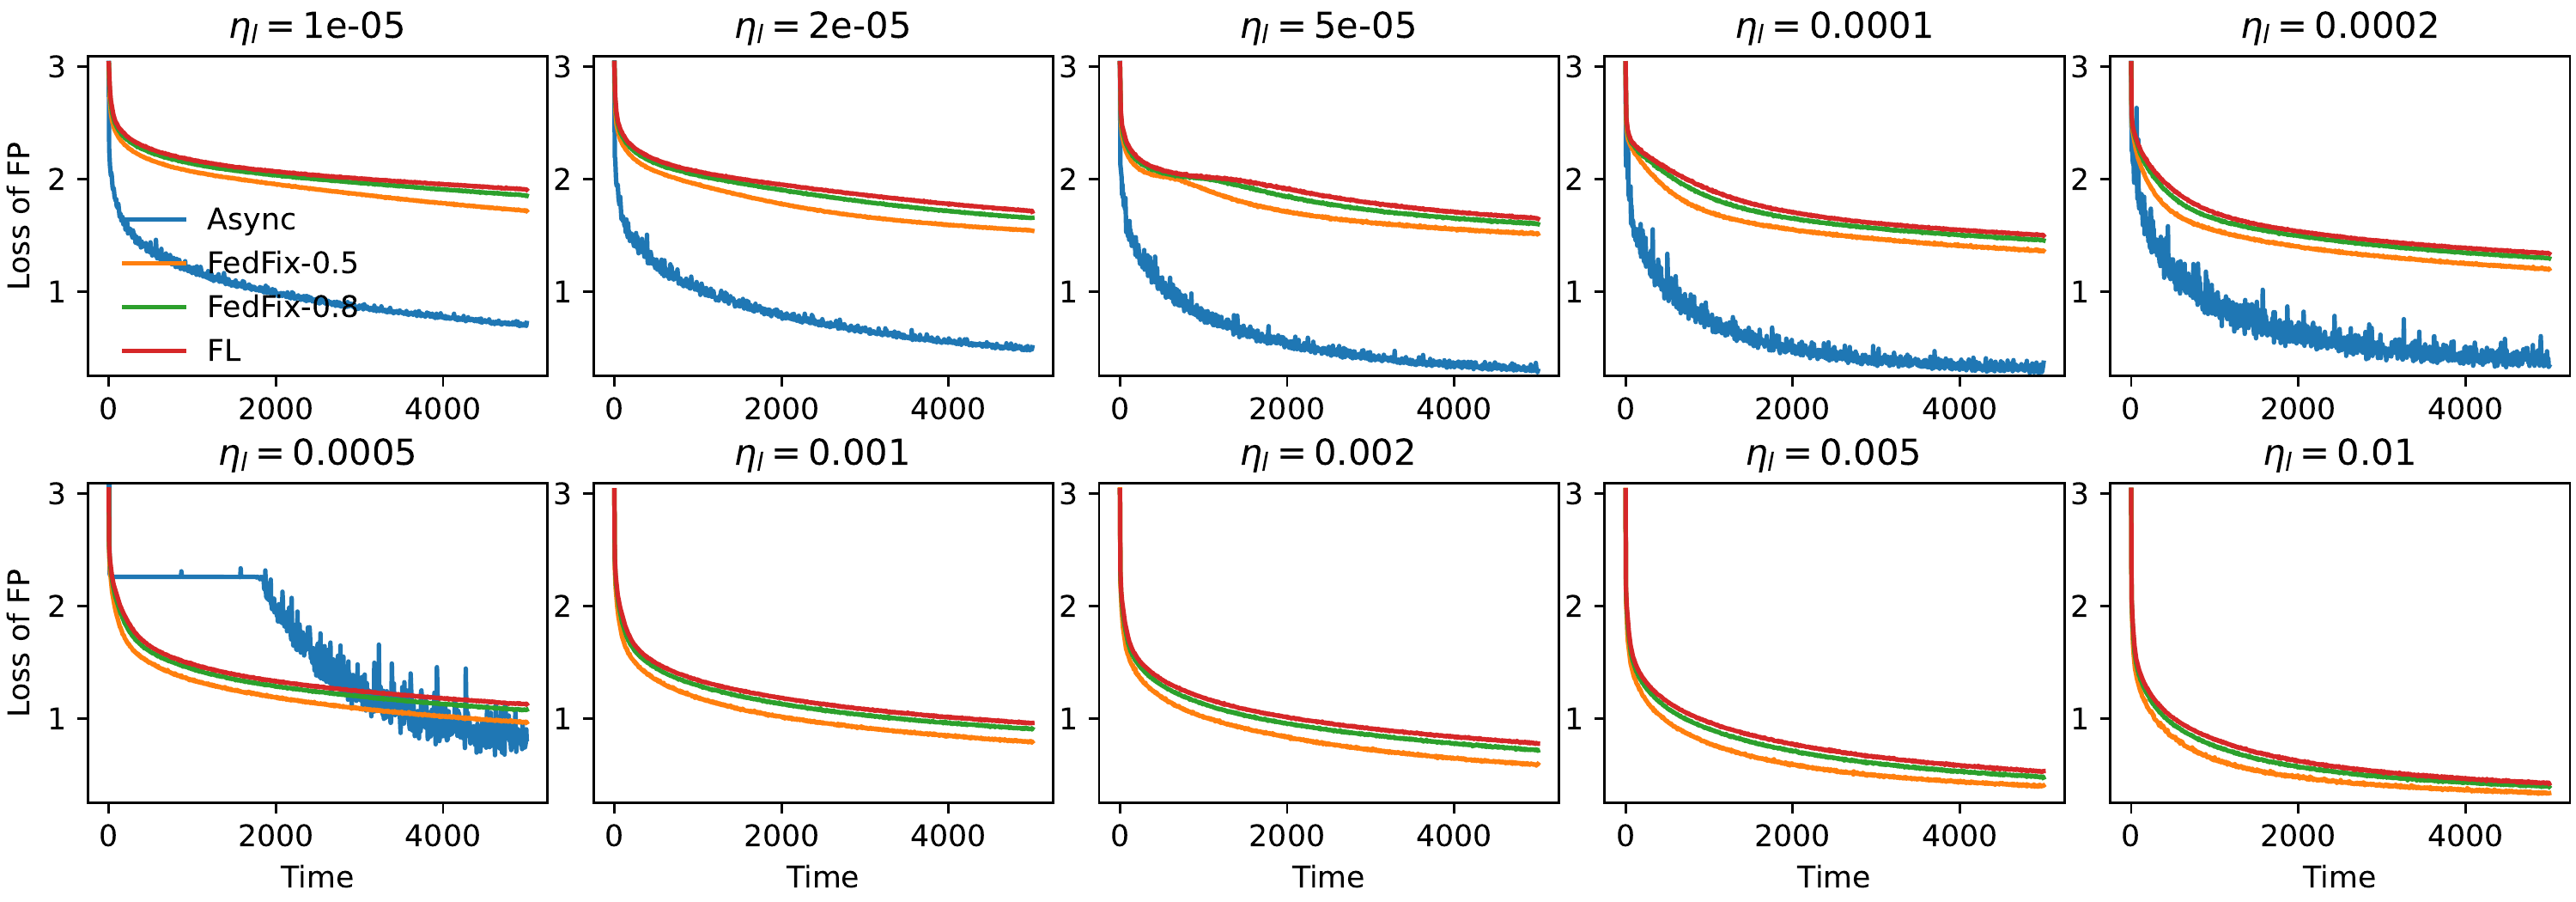}
	\caption{Evolution of federated problem (\ref{eq:original_problem_general}) loss for CIFAR10 and time scenario $F80$ with $M=50$ and $K = 10$.}
	\label{app:fig:explore_CIFAR10_50}
\end{figure}

\begin{figure}
	\centering
	\includegraphics[width=\linewidth]{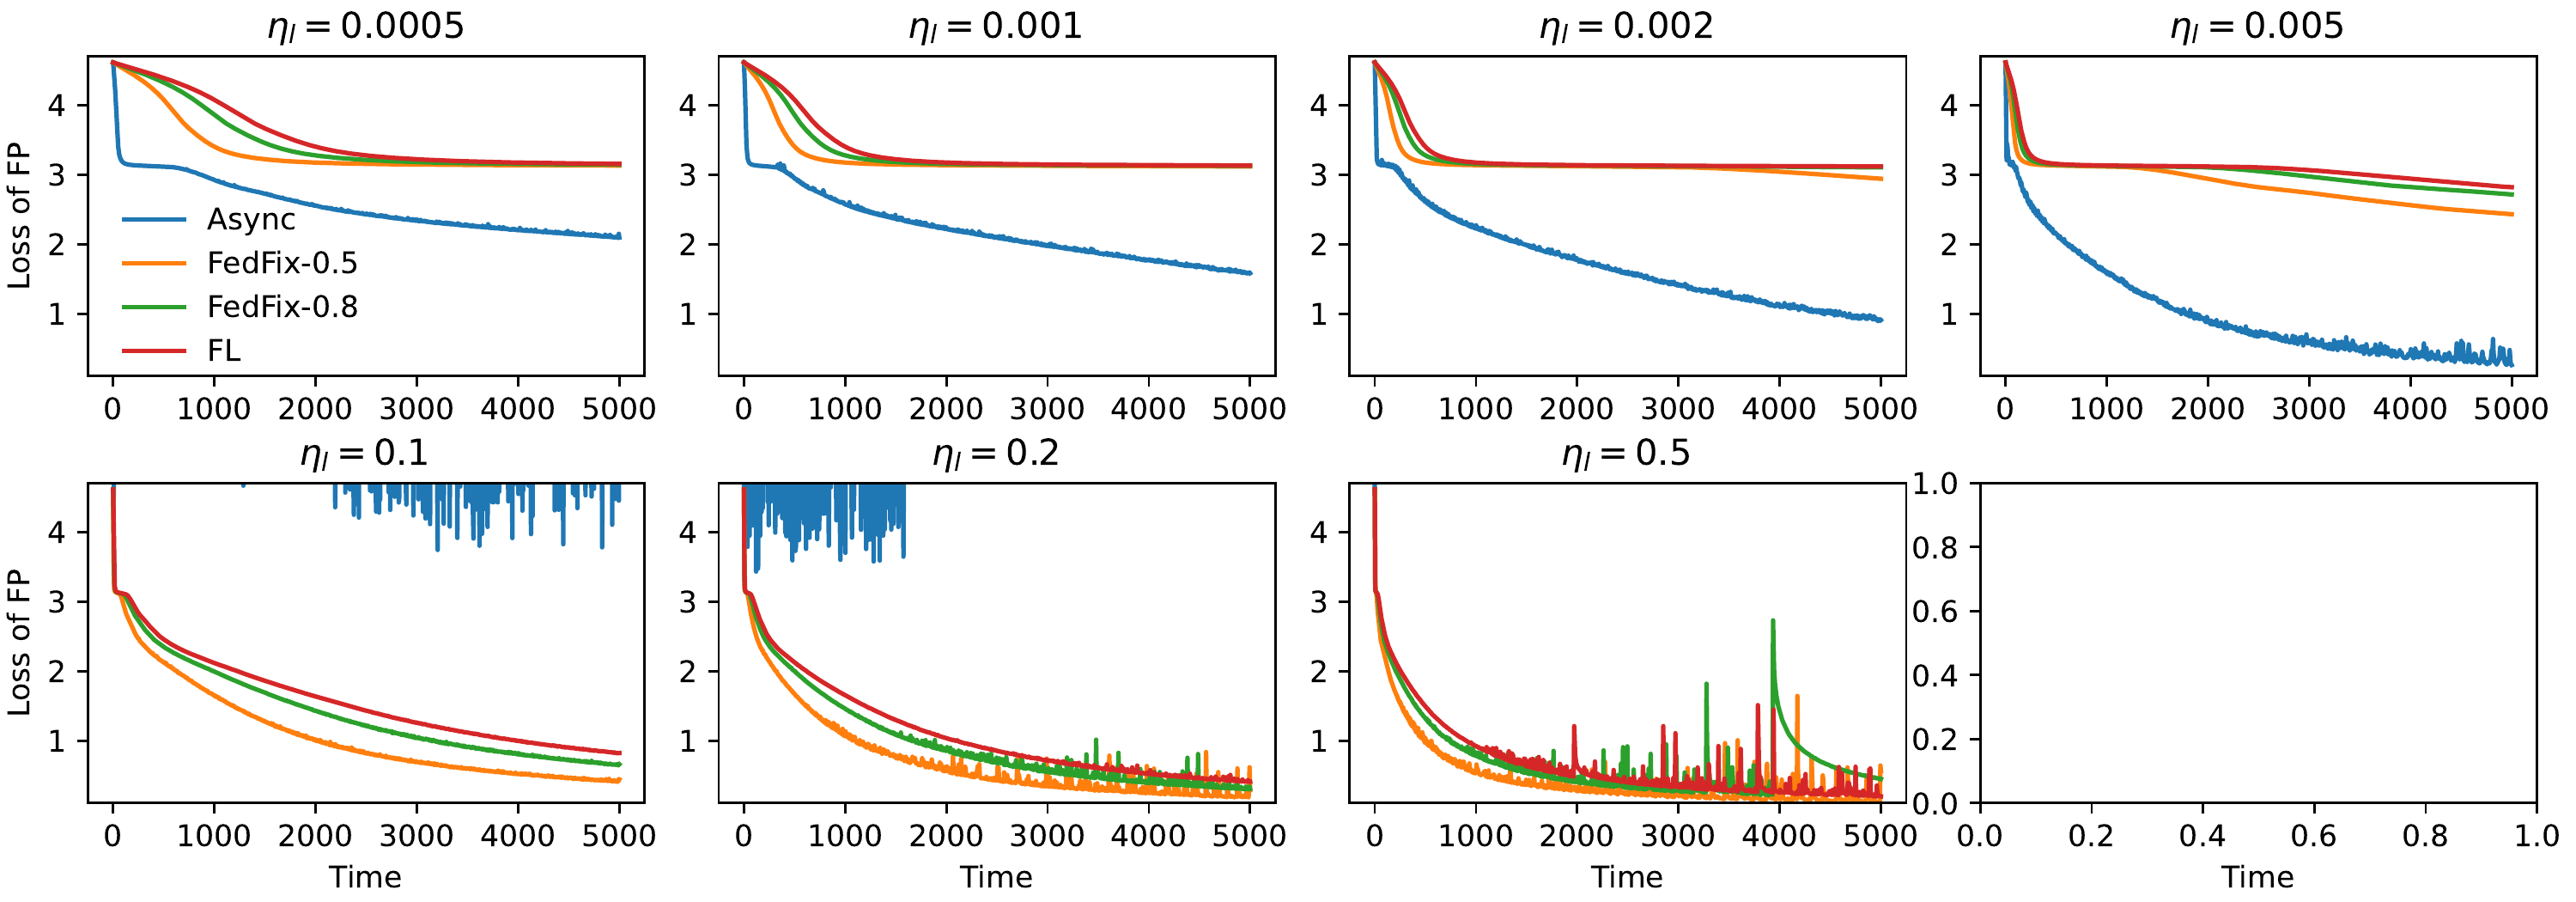}
	\caption{Evolution of federated problem (\ref{eq:original_problem_general}) loss for Shakespeare and time scenario $F80$ with $M=20$ and $K = 10$.}
	\label{app:fig:explore_Shakespeare_20}
\end{figure}
